# Supplementary material for: NOMU: Neural Optimization-based Model Uncertainty
Source: arXiv:2102.13640 source file (2023-03-11)

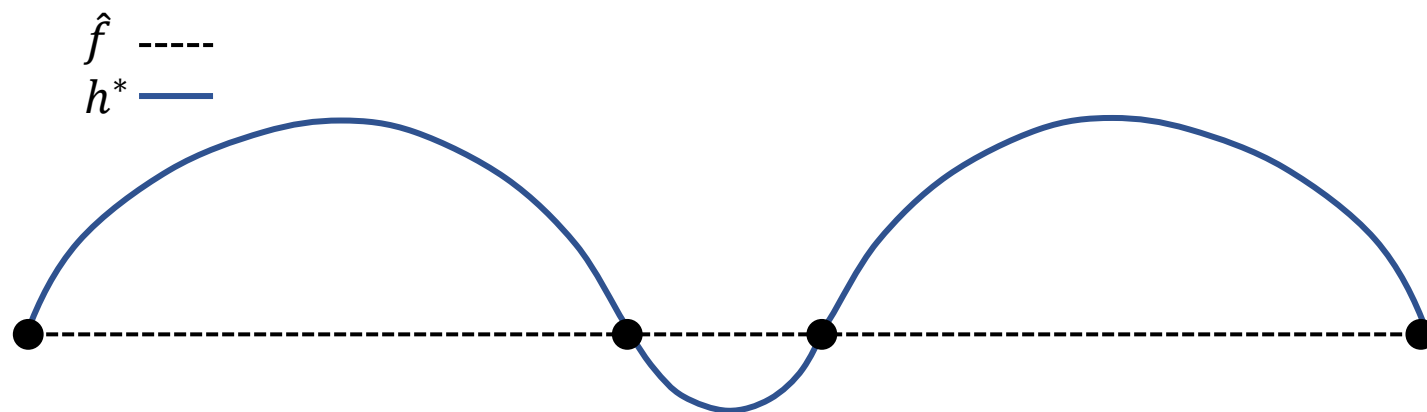

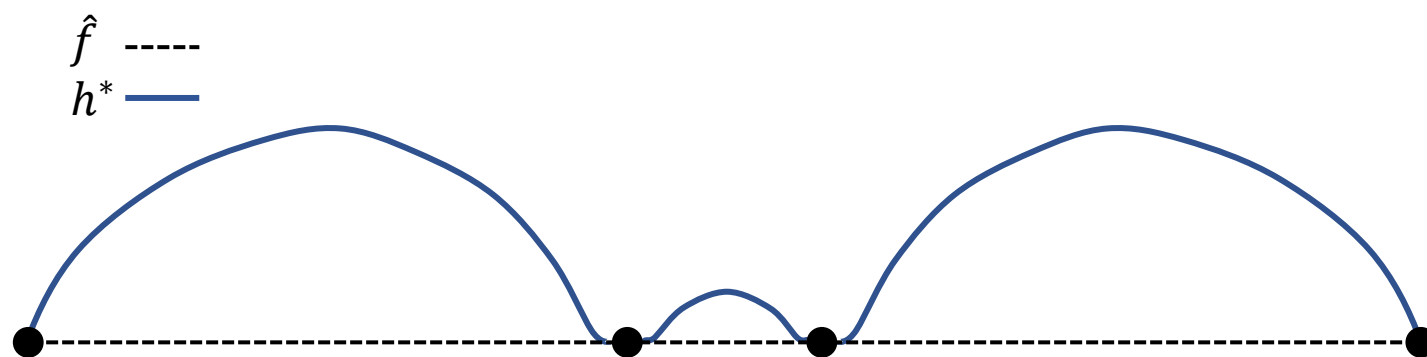

Supplement: Supplementary file 1 [file motivation_exponential_u.pdf]
